# Supplementary material for: Zero-Label Prompt Selection
Source: arXiv:2211.04668 source file (2022-11-09)
Supplement: Supplementary file 1 [file 6_appendix.tex]

\appendix
\section{Appendix}

\subsection{XXXX}
